# Supplementary material for: Better plain ViT baselines for ImageNet-1k
Source: arXiv:2205.01580 source file (2022-05-03)
Supplement: Supplementary file 1 [file appendix.tex]

\appendix

\section{Full results tables}\label{sec:app:table}

We provide a full summary of our experiments on ImageNet in Table~\ref{tbl:models}, with a dash ``-'' marking settings we did not deem necessary to run, as the cost outweights the potential insights.

Furthermore, Table~\ref{tbl:patience} gives numerical results for the models shown in Figure~\ref{fig:patience}, our best models (according to validation) on the four smaller datasets at $128$px resolution, together with baselines and the teacher.

\begin{table*}[t]
  \setlength{\tabcolsep}{0pt}
  \setlength{\extrarowheight}{5pt}
  
  \newcolumntype{C}{>{\centering\arraybackslash}X}
  \newcolumntype{R}{>{\raggedleft\arraybackslash}X}
  \centering
  \vspace{-2em}
  \caption{Summary of all ImageNet distillation runs. Numbers represent top-1 accuracy on the validation set. By default, the student is always a ResNet50 and the teacher is BiT-M-R152x2.}\label{tbl:models}
  % Format is type{width}, p: paragraph, top-align, C is custom, c is squeezed.
  % NOTE: No phantom here as it messes up on arxiv...
  \begin{tabularx}{\linewidth}{p{5.4cm}p{0.1cm}Cp{0.01cm}Cp{0.01cm}Cp{0.01cm}Cp{0.01cm}Cp{0.01cm}Cp{0.01cm}C}
    \toprule[1pt]
    \bf{Experiment} && \bf{30ep} && \bf{90ep} && \bf{300ep} && \bf{600ep} && \bf{1200ep} && \bf{4800ep} && \bf{9600ep} \\
    \midrule
Best from labels     &&   -   && 76.59 && 78.08 &&   -   && 78.15 && 76.59 &&   -   \\
Fixed teacher        && 73.75 && 76.45 && 77.76 && 77.99 && 78.11 && 77.56 && 76.95 \\
consistent teacher   && 74.95 && 78.05 && 80.08 && 80.63 && 81.15 && 81.58 && 81.76 \\
function matching (FunMatch) && 73.89 && 78.00 && 80.30 && 81.17 && 81.54 && 82.18 && 82.31 \\
    \midrule
consistent teacher \shampoo     && 75.45 && 78.79 && 80.54 && 81.11 && 81.44 &&   -   &&   -   \\
function matching \shampoo       && 75.12 && 78.70 && 80.63 &&   -   && 81.67 &&   -   &&   -   \\
    \midrule
T224 $\rightarrow$ S160 (consistent teacher)  && 71.38 && 75.57 && 78.01 &&   -   &&   -   &&   -   &&   -   \\
T224 $\rightarrow$ S160 (function matching)   && 70.22 && 75.34 && 78.17 && 79.07 && 79.61 &&  0.10 && 80.49 \\
    \arrayrulecolor{lightgray}\midrule[0.25pt]\arrayrulecolor{black}
FunMatch: T384 $\rightarrow$ S224          &&   -   &&   -   && 80.46 &&   -   && 81.82 && 82.33 && 82.64 \\
    \arrayrulecolor{lightgray}\midrule[0.25pt]\arrayrulecolor{black}
FunMatch: T384+224 $\rightarrow$ S224      &&   -   &&   -   &&   -   &&   -   && 82.12 && 82.71 && 82.82 \\
% T384+224 $\rightarrow$ S224 \shampoo &&   -   &&   -   &&   -   &&   -   && 82.24 && 82.76 &&  \T{WIP}  \\
    \midrule
FunMatch: MobileNet v3 (GN)    &&   -   &&   -   && 74.60 &&   -   && 76.31 && 76.84 && 76.97 \\
FunMatch: MobileNet v3 (GN, 2T) &&   -   &&   -   && 74.85 &&   -   && 76.51 &&   -   &&   -   \\
FunMatch: MobileNet v3 (GN, Small) &&   -   &&   -   && 65.61 &&   -   && 67.57 &&   -   &&   -   \\
    \arrayrulecolor{lightgray}\midrule[0.25pt]\arrayrulecolor{black}
FunMatch: MobileNet v3 (BN)    &&   -   &&   -   && 72.32 &&   -   && 73.51 &&   -   &&   -   \\
FunMatch: MobileNet v3 (BN, 2T) &&   -   &&   -   && 73.28 &&   -   &&   -   &&   -   &&   -   \\
    \midrule
Figure~\ref{fig:imagenet} (right): BiT-M-R50 init       && 77.52 && 79.43 && 80.47 && 80.83 && 81.11 && 81.45 &&   -   \\
Figure~\ref{fig:imagenet_baselines}: SGDM && - && 76.59 && 76.38 && - && 74.93 && 73.48 && - \\
Figure~\ref{fig:imagenet_baselines}: Adam && - && 74.92 && 74.55 && - && 73.47 && 70.66 && - \\
Figure~\ref{fig:imagenet_baselines}: SGDM + Mixup && - && 76.18 && 78.06 && - && 75.01 && 71.40 && - \\
Figure~\ref{fig:imagenet_baselines}: Adam + Mixup && - && 76.17 && 78.08 && - && 78.15 && 76.59 && - \\
    \bottomrule
  \end{tabularx}
  %\vspace{-2em}
\end{table*}

\begin{table*}[t]
  \setlength{\tabcolsep}{5pt}
  \setlength{\extrarowheight}{5pt}
  
  \centering
  \caption{Tabular representation of the results from Figure~\ref{fig:patience}.}\label{tbl:patience}
  % Format is type{width}, p: paragraph, top-align, C is custom, c is squeezed.
  % \begin{tabularx}{\linewidth}{p{3cm}p{0.1cm}Rp{0.01cm}Cp{0.01cm}Rp{0.01cm}Cp{0.01cm}Cp{0.01cm}Lp{0.01cm}L}
  % \begin{tabulary}{\textwidth}{LS[table-format=6.3]
  \begin{tabulary}{1.0\textwidth}{LRCRLL}
    \toprule[1pt]
    %\bf{Model} && \centering \bf{Epochs} && \bf{Final Test Acc} && \centering \bf{T} && \bf{LR} && \bf{WD} \\
    \bf{Model} & \centering \bf{Epochs} & \bf{Final Test Acc} & \centering \bf{T} & \bf{LR} & \bf{WD} \\
\midrule
\midrule
\multicolumn{6}{c}{\emph{Flowers102}} \\
\arrayrulecolor{lightgray}\midrule[0.25pt]\arrayrulecolor{black}
ResNet-50x1 student        &        1000 & 77.51\% & 10 &   0.003 & 0.001 \\
ResNet-50x1 student        &     10\,000 & 92.83\% & 10 &   0.003 & 0.0003 \\
ResNet-50x1 student        &    100\,000 & 95.54\% &  1 &   0.001 & 0.0001 \\
ResNet-50x1 student        & 1\,000\,000 & 96.93\% &  1 &  0.0003 & 1e-05 \\
\arrayrulecolor{lightgray}\midrule[0.25pt]\arrayrulecolor{black}
ResNet-152x2 teacher       & - & 97.82\% & - & - & - \\
Best transfer ResNet50     &     10\,000 & 97.50\% & \multicolumn{3}{c}{LR=0.01, Mixup=0.0}  \\
Best from-scratch ResNet50 &     10\,000 & 66.38\% & \multicolumn{3}{c}{LR=0.01, Mixup=1.0}  \\
\midrule
\multicolumn{6}{c}{\emph{Pet37}} \\
\arrayrulecolor{lightgray}\midrule[0.25pt]\arrayrulecolor{black}
ResNet-50x1 student        &         300 & 82.75\% &  2 &    0.01 & 1e-05 \\
ResNet-50x1 student        &        1000 & 88.01\% &  5 &    0.01 & 0.001 \\
ResNet-50x1 student        &        3000 & 90.08\% & 10 &   0.003 & 0.0003 \\
ResNet-50x1 student        &     10\,000 & 90.98\% &  2 &   0.001 & 0.0001 \\
ResNet-50x1 student        &     30\,000 & 91.06\% &  2 &   0.003 & 1e-05 \\
\arrayrulecolor{lightgray}\midrule[0.25pt]\arrayrulecolor{black}
ResNet-152x2 teacher       & - & 91.03\% & - & - & - \\
Best transfer ResNet50     &     10\,000 & 88.20\% & \multicolumn{3}{c}{LR=0.001, Mixup=1.0}  \\
Best from-scratch ResNet50 &     10\,000 & 74.24\% & \multicolumn{3}{c}{LR=0.01, Mixup=1.0}  \\
\midrule
\multicolumn{6}{c}{\emph{Food101}} \\
\arrayrulecolor{lightgray}\midrule[0.25pt]\arrayrulecolor{black}
ResNet-50x1 student        &         100 & 83.29\% & 10 &    0.01 & 0.001 \\
ResNet-50x1 student        &        1000 & 86.64\% & 10 &   0.001 & 0.0003 \\
ResNet-50x1 student        &        3000 & 87.20\% &  5 &    0.01 & 0.0001 \\
\arrayrulecolor{lightgray}\midrule[0.25pt]\arrayrulecolor{black}
ResNet-152x2 teacher       & - & 86.24\% & - & - & - \\
Best transfer ResNet50     &        1000 & 85.05\% & \multicolumn{3}{c}{LR=0.001, Mixup=1.0}  \\
Best from-scratch ResNet50 &        1000 & 74.56\% & \multicolumn{3}{c}{LR=0.01, Mixup=1.0}  \\
\midrule
\multicolumn{6}{c}{\emph{Sun397}} \\
\arrayrulecolor{lightgray}\midrule[0.25pt]\arrayrulecolor{black}
ResNet-50x1 student        &         100 & 68.28\% & 10 &    0.01 & 0.001 \\
ResNet-50x1 student        &        1000 & 73.46\% & 10 &   0.003 & 0.0001 \\
ResNet-50x1 student        &        3000 & 74.26\% & 10 &    0.01 & 3e-05 \\
\arrayrulecolor{lightgray}\midrule[0.25pt]\arrayrulecolor{black}
ResNet-152x2 teacher       & - & 74.22\% & - & - & - \\
Best transfer ResNet50     &        1000 & 71.61\% & \multicolumn{3}{c}{LR=0.001, Mixup=1.0} \\
Best from-scratch ResNet50 &        1000 & 60.63\% & \multicolumn{3}{c}{LR=0.01, Mixup=1.0}  \\
    \bottomrule
  % \end{tabularx}
  \end{tabulary}
  %\vspace{-2em}
\end{table*}

\section{BiT models download statistics}\label{sec:app:download}

\begin{figure*}[ht]%
    \centering
    \includegraphics[width=\textwidth]{figs/appendix/download_statistics.pdf}
    %\vspace{-1em}
    \caption{
      BiT models download statistics according to \url{https://tfhub.dev/google/collections/bit}.
      ``BiT-S''/``BiT-M'' denotes the BiT model for feature extraction, 
      while the figures with a mention of ``head'' correspond to the classifiers.
      The rightmost overall plot shows the total download counts for each size. 
      It is clear that ResNet-50 is by far the most widely used model.
    }%
    %\vspace{-1em}
    \label{fig:app:download}%
\end{figure*}

In Figure~\ref{fig:app:download}, we show the download statistics for models with different sizes: ResNet50, ResNet50x3, ResNet101, ResNet101x3 and ResNet152x4. 
It's clear that the smallest ResNet50 model is the most used, with a significant gap compared to the other models.
The practitioners' behavior motivates our work of getting the best possible ResNet50 model.

\section{More consistency plots}\label{sec:app:consistency}

In Figures~\ref{fig:app:consistency_flowers}~to~\ref{fig:app:consistency_sun}, we show the ``consistency'' plots (cf Figure~\ref{fig:consistency} in the main paper) for all datasets and across all training durations.
It is noteworthy that (relatively) short runs may provide deceptive signal on the best method, and only with the addition of ``patience'', \eg when distilling for a long time, does it become clear that the full function-matching approach is the best choice.
\section{Shampoo optimization details}\label{sec:app:shampoo}
For all experiments the learning rate schedule was a linear warm-up up to 1800 steps followed by a quadratic decay towards zero. Overhead of Shampoo is quite minimal due blocking trick (each preconditioner is atmost 128x128) and inverse is run in a distributed manner across the TPU cores every step, with nesterov momentum. These settings are identical to the the training recipe in \cite{anil2021scalable} for training a ResNet-50 architecture on ImageNet from scratch efficiently at large batch sizes.  All experiments uses weight decay of 0.000375. 

\section{Training, validation and test splits}\label{app:splits}

\begin{table*}[t]
  \setlength{\tabcolsep}{0pt}
  \setlength{\extrarowheight}{5pt}
  
  \newcolumntype{C}{>{\centering\arraybackslash}X}
  \newcolumntype{R}{>{\raggedleft\arraybackslash}X}
  \centering
  \caption{\emph{Train}, \emph{validation} and \emph{test} splits. Split definitions follow notation from the \emph{tensorflow datasets} library and can be directly used to access relevant data splits using the library.}\label{tbl:splits}
  \vspace{1mm}
  \begin{tabularx}{\linewidth}{p{2.3cm}p{0.1cm}Cp{0.01cm}Cp{0.01cm}Cp{0.01cm}C}
    \toprule[1pt]
    \bf{Dataset} && \bf{train split} && \bf{validation split} && \bf{test split} \\
    \midrule
    Flowers102 && \texttt{train} && \texttt{validation} && \texttt{test} \\
    Pets37 &&  \texttt{train[:90}\%\texttt{]} &&  \texttt{train[90}\%\texttt{:]} &&  \texttt{test} \\
    Food101 &&  \texttt{train[:90}\%\texttt{]} &&  \texttt{train[90}\%\texttt{:]} &&  \texttt{test} \\
    Sun397 && \texttt{train} && \texttt{validation} && \texttt{test} \\
    ImageNet &&  \texttt{train[:98}\%\texttt{]} &&  \texttt{train[98}\%\texttt{:]} &&  \texttt{validation} \\
    \bottomrule
  \end{tabularx}
\end{table*}

Throughout our experiments we rely on the \emph{tensorflow datasets} library\footnote{\url{https://www.tensorflow.org/datasets}} to access all datasets. A huge advantage of this library is that it enables a unified and reproducible way to access diverse datasets. To this end, we report our \emph{train}, \emph{validation} and \emph{test} splits (following the library's notation) in Table~\ref{tbl:splits}.

\begin{figure*}[ht]%
    \centering
    \includegraphics[width=\textwidth]{figs/appendix/flowers_1k.pdf}
    \includegraphics[width=\textwidth]{figs/appendix/flowers_10k.pdf}
    \includegraphics[width=\textwidth]{figs/appendix/flowers_100k.pdf}
    %\vspace{-1em}
    \caption{Consistency plots for the Flowers102 dataset, when training for 1\,000~epochs, 10\,000~epochs, and 100\,000~epochs, from top to bottom respectively.}%
    %\vspace{-1em}
    \label{fig:app:consistency_flowers}%
\end{figure*}

\begin{figure*}[ht]%
    \centering
    \includegraphics[width=\textwidth]{figs/appendix/pets_1k.pdf}
    \includegraphics[width=\textwidth]{figs/appendix/pets_3k.pdf}
    \includegraphics[width=\textwidth]{figs/appendix/pets_10k.pdf}
    \includegraphics[width=\textwidth]{figs/appendix/pets_30k.pdf}
    %\vspace{-1em}
    \caption{Consistency plots for the Pet37 dataset, when training for 1\,000~epochs, 3\,000~epochs, 10\,000~epochs, and 30\,000~epochs, from top to bottom respectively.}%
    %\vspace{-1em}
    \label{fig:app:consistency_pets}%
\end{figure*}

\begin{figure*}[ht]%
    \centering
    \includegraphics[width=\textwidth]{figs/appendix/food_100.pdf}
    \includegraphics[width=\textwidth]{figs/appendix/food_1k.pdf}
    \includegraphics[width=\textwidth]{figs/appendix/food_3k.pdf}
    %\vspace{-1em}
    \caption{Consistency plots for the Food101 dataset, when training for 100~epochs, 1\,000~epochs, and 3\,000~epochs, from top to bottom respectively.}%
    %\vspace{-1em}
    \label{fig:app:consistency_food}%
\end{figure*}

\begin{figure*}[ht]%
    \centering
    \includegraphics[width=\textwidth]{figs/appendix/sun_100.pdf}
    \includegraphics[width=\textwidth]{figs/appendix/sun_1k.pdf}
    \includegraphics[width=\textwidth]{figs/appendix/sun_3k.pdf}
    %\vspace{-1em}
    \caption{Consistency plots for the SUN397 dataset, when training for 100~epochs, 1\,000~epochs, and 3\,000~epochs, from top to bottom respectively.}%
    %\vspace{-1em}
    \label{fig:app:consistency_sun}%
\end{figure*}
